# Supplementary material for: The large-scale structure of globular clusters in the NGC 1052 group
Source: arXiv:2303.16375 source file (2023-03-29)
Supplement: Supplementary file 1 [file appendixA.tex]

% \section{The GC distribution in NGC 1052}
% \label{sec:appendixA}

% In Fig. \ref{fig:GC_dist}, we show the positions of every GC candidate selected according to the criteria described in Section \ref{sec:GC}.

% \begin{figure*}
%     \centering
%     \includegraphics[width=\textwidth]{Fig/distribution_GCs_scatter_smallcellsize.png}
%     \caption{GC candidates positions across the NGC 1052 group. Red points are the GC candidates, green triangles are the galaxies in the ``bullet'' trail proposed by \protect\cite{vanDokkum_22}. The black ellipse is the half-light radius found for the total GC distribution of the central galaxy, NGC 1052. Blue and red ellipses are the half-light radius for the blue and red GC distribution respectively. All points are overplotted in the combined CFHT $g$ ban image of the group NGC 1052.}
%     \label{fig:GC_dist}
% \end{figure*}
